# Supplementary material for: ARIANN: Low-Interaction Privacy-Preserving Deep Learning via Function Secret Sharing
Source: arXiv:2006.04593 source file (2021-10-28)
Supplement: Supplementary file 1 [file E_extra_experiments.tex]

\begin{table*} 
\caption{Comparison of the inference time between secure frameworks on several popular network architectures. Time is reported in seconds in the LAN and WAN setting, and communication in MB.\label{table:old_inference}}
\vspace*{-.111cm}
\begin{center}
\begin{tabular}{l c c c c c c c c c c c}
\hline
  & & & \multicolumn{3}{c}{Network-1} & \multicolumn{3}{c}{Network-2} & \multicolumn{3}{c}{LeNet}\\ 
Framework & Dataset & Processor & LAN   & WAN   & Comm. & LAN   & WAN   & Comm. & LAN   & WAN   & Comm. \\
\hline
\textit{AriaNN (preprocessing)} & MNIST & CPU & 0.002 & 0.014 & 0.36 & 0.028 & 0.626 & 9.98 & 0.041 & 0.997 & 14.66 \\
AriaNN (online phase)          & MNIST  & CPU & 0.004 & 0.043 & 0.022 & 0.041 & 0.133 & 0.28 & 0.055 & 0.143 & 0.43 \\
% Previous versions AriaNN (CPU + onl    &    & 0.004 & 0.055 & 0.013 & 0.094 & 0.234 & 0.33 & 0.129 & 0.289 & 0.46 \\
\textit{AriaNN (preprocessing)} \kern-1em  & MNIST  & GPU & 0.006 & x & x & 0.068 & x & x & 0.101 & x & x \\
AriaNN (online phase)\kern-1em             & MNIST & GPU & 0.002 & x & x & 0.024 & x & x & 0.035 & x & x \\
FALCON    & MNIST   & CPU & 0.011 & 0.990 & 0.012 & 0.009 & 0.76  & 0.049  & 0.047 & 3.06  & 0.74 \\
SecureNN  & MNIST   & CPU & 0.043 & 2.43  & 2.1   & 0.130 & 3.93  & 8.86  & -     & -     & -    \\
XONN      & MNIST   & CPU & 0.130 & -     & 4.29  & 0.150 & -     & 32.1  & -     & -     & -    \\
Gazelle   & MNIST   & CPU & 0.090  & -     & 0.5   & 1.16  & -     & 70    & -     & -     & -    \\
$\textrm{ABY}^3$& MNIST & CPU & 0.008 & - & 0.5   & -     & -     & -     & -     & -     & -    \\
\hline
\end{tabular}

\vspace*{0.1cm}

\begin{tabular}{l c c c c c c c c c c c}
\hline
 & & & \multicolumn{3}{c}{AlexNet} & \multicolumn{3}{c}{VGG16} & \multicolumn{3}{c}{ResNet18}\\ 
Framework & Dataset & Processor & LAN   & WAN   & Comm. & LAN   & WAN   & Comm. & LAN   & WAN   & Comm. \\
\hline
\textit{AriaNN (preprocessing)} & CIFAR-10 & CPU & 
              0.09 & 2.17 & 24.63 & 0.94 & 53.92 & 276.86 & - & - & - \\
AriaNN (online phase)           & CIFAR-10 & CPU &
              0.15 & 0.34 & 0.95  & 1.75 & 1.99 & 12.59 & - & - & - \\
\textit{AriaNN (preprocessing)} & CIFAR-10 & GPU & 
              0.163 & x & x & 1.98 & x & x  & - & - & - \\ % VGG16 GPU batch_size = 14
AriaNN (online phase)           & CIFAR-10 & GPU &
              0.078 & x & x & 1.55 & x & x  & - & - & - \\
FALCON    & CIFAR-10 & CPU &
              0.043 & 0.13 & 1.35 & 0.79 & 1.27 & 13.51 & - & - & - \\
\textit{AriaNN (preprocessing)} & $\!\!\!\!\!\!\!\!\small{64\!\times\!64}$ ImageNet\!\!\!\!  & CPU & 
              0.27 & 23.86 & 88.40 & 3.42 & 214.74 & 1123.81 & - & - & - \\
AriaNN (online phase) & $\!\!\!\!\!\!\!\!\small{64\!\times\!64}$ ImageNet\!\!\!\!  & CPU & 
              0.33 & 0.48 & 1.75 & 7.51 & 8.00 & 53.11 & - & - & - \\
FALCON    & $\!\!\!\!\!\!\!\!\small{64\!\times\!64}$ ImageNet\!\!\!\!  & CPU & 
              1.81 & 2.43 & 19.21 & 3.15 & 4.67 & 52.56 & - & - & - \\
\textit{AriaNN (preprocessing)} & $\!\!\!\!\!\!\!\!\small{224\!\times\!224}$ Hymenoptera\!\!\!\!\!\! & CPU & 
             - & - & - & - & - & - &  10.02 & 905.11 & 3254 \\
AriaNN (online phase)           & $\!\!\!\!\!\!\!\!\small{224\!\times\!224}$ Hymenoptera\!\!\!\!\!\! & CPU & 
             - & - & - & - & - & - &  19.88  & 24.07 & 148 \\
\textit{AriaNN (preprocessing)} & $\!\!\!\!\!\!\!\!\small{224\!\times\!224}$ Hymenoptera\!\!\!\!\!\! & GPU & 
             - & - & - & - & - & - &  22.56 & x & x \\ % ResNet18 GPU batch_size = 1
AriaNN (online phase)           & $\!\!\!\!\!\!\!\!\small{224\!\times\!224}$ Hymenoptera\!\!\!\!\!\! & GPU & 
             - & - & - & - & - & - &  13.90 & x & x \\
\hline
\end{tabular}

% Resnet18: BS = 8
% VGG CIFAR10: 64
% VGG Tiny Imagenet: 16 (all 32 -> 7.1s ; all 64 -> 6.48)

\vspace*{-.322cm}
\end{center}
\end{table*}
